# Supplementary material for: Lock-Free Locks Revisited
Source: arXiv:2201.00813 source file (2022-01-28)
Supplement: Supplementary file 1 [file list-appendix.tex]

\section{List code}

Following up on the example from Section~\ref{sec:listexample}
Figure~\ref{alg:listext} shows the code for insert and find.

\begin{figure}
\begin{lstlisting}
void insert(link* head, K k, V v) {
	while (true) {
		auto [cur, nxt] = find_location(head, k);
		if (nxt->k == k) return;
		if (try_lock(cur->lck, [=] () {
				if (cur->removed.load() ||
				  (cur->next).load() != nxt) return false;
				link* new_link = link_pool.allocate(k, v, nxt);
				cur->next = new_link;
				return true;}))
			return;}}

std::optional<V> find(link* head, K k) {
	link* nxt = (head->next).load();
	while (k > nxt->key) nxt = (nxt->next).load();
	if (nxt->key == k) return nxt->value; 
	else return {};}
\end{lstlisting}
\caption{Insertion and Find for lazy lists~\cite{lazylist06}}
\label{alg:listext}
\end{figure}
